# Supplementary material for: Measurement of the lifetimes of promptly produced $\Omega^{0}_{c}$ and $\Xi^{0}_{c}$ baryons
Source: arXiv:2109.01334 source file (2022-02-28)
Supplement: Supplementary file 1 [file supplementary.tex]

\clearpage
\section*{Supplementary material}

An illustration of the \lhcb measurements of \Omegac and \Xicz lifetimes 
and the previous world average is shown in Fig.~\ref{fig:result},
and the fit projections to the invariant mass and \logchisqip distributions
in different decay-time intervals and data-taking periods are shown in Fig.~6--29.

\begin{figure}[htb]
  \centering
  \includegraphics[width=0.80\linewidth]{Fig1_S.pdf}
  \caption{Illustration of the \lhcb measurements of the \Omegac and \Xicz lifetimes 
  obtained from semileptonic beauty-hadron decays~\cite{LHCb-PAPER-2018-028,LHCb-PAPER-2019-008}
  and prompt signals,
  and the previous 2018 world average~\cite{PDG2018}.
  The combined \lhcb results are shown in coloured bands.}
  \label{fig:result}
\end{figure}

%%%%%%%%%%%%%%%%%%%%%%%%%%%%%%%%%%%%%%%%%%%%%%%%%%%%%%%%%%%%%%
% For Omegac/Xic/Dz and 16/17/18 and 1/2/3 decay-time interval
%%%%%%%%%%%%%%%%%%%%%%%%%%%%%%%%%%%%%%%%%%%%%%%%%%%%%%%%%%%%%%
\begin{figure}[tb]
  \centering
  \includegraphics[width=0.45\linewidth]{Fig2a_S.pdf}
  \includegraphics[width=0.45\linewidth]{Fig2b_S.pdf}
\caption{
Distributions of (left) invariant mass and (right) \logchisqip in the reduced mass region of $[2683,2707]\mevcc$ for the \Omegac data sample collected in 2016\ in the decay-time interval of $[0.52,0.57]\ps$, along with the fit results.  The contributions of the signal, the secondary decays, and the combinatorial background are shown in red (solid), green (dashed), and gray (dash-dotted), respectively.
}
\end{figure}

\begin{figure}[tb]
  \centering
  \includegraphics[width=0.45\linewidth]{Fig3a_S.pdf}
  \includegraphics[width=0.45\linewidth]{Fig3b_S.pdf}
\caption{
Distributions of (left) invariant mass and (right) \logchisqip in the reduced mass region of $[2683,2707]\mevcc$ for the \Omegac data sample collected in 2016\ in the decay-time interval of $[0.69,0.75]\ps$, along with the fit results.  The contributions of the signal, the secondary decays, and the combinatorial background are shown in red (solid), green (dashed), and gray (dash-dotted), respectively.
}
\end{figure}

\begin{figure}[tb]
  \centering
  \includegraphics[width=0.45\linewidth]{Fig4a_S.pdf}
  \includegraphics[width=0.45\linewidth]{Fig4b_S.pdf}
\caption{
Distributions of (left) invariant mass and (right) \logchisqip in the reduced mass region of $[2683,2707]\mevcc$ for the \Omegac data sample collected in 2016\ in the decay-time interval of $[0.9,1.05]\ps$, along with the fit results.  The contributions of the signal, the secondary decays, and the combinatorial background are shown in red (solid), green (dashed), and gray (dash-dotted), respectively.
}
\end{figure}

\begin{figure}[tb]
  \centering
  \includegraphics[width=0.45\linewidth]{Fig5a_S.pdf}
  \includegraphics[width=0.45\linewidth]{Fig5b_S.pdf}
\caption{
Distributions of (left) invariant mass and (right) \logchisqip in the reduced mass region of $[2683,2707]\mevcc$ for the \Omegac data sample collected in 2017\ in the decay-time interval of $[0.52,0.57]\ps$, along with the fit results.  The contributions of the signal, the secondary decays, and the combinatorial background are shown in red (solid), green (dashed), and gray (dash-dotted), respectively.
}
\end{figure}

\begin{figure}[tb]
  \centering
  \includegraphics[width=0.45\linewidth]{Fig6a_S.pdf}
  \includegraphics[width=0.45\linewidth]{Fig6b_S.pdf}
\caption{
Distributions of (left) invariant mass and (right) \logchisqip in the reduced mass region of $[2683,2707]\mevcc$ for the \Omegac data sample collected in 2017\ in the decay-time interval of $[0.69,0.75]\ps$, along with the fit results.  The contributions of the signal, the secondary decays, and the combinatorial background are shown in red (solid), green (dashed), and gray (dash-dotted), respectively.
}
\end{figure}

\begin{figure}[tb]
  \centering
  \includegraphics[width=0.45\linewidth]{Fig7a_S.pdf}
  \includegraphics[width=0.45\linewidth]{Fig7b_S.pdf}
\caption{
Distributions of (left) invariant mass and (right) \logchisqip in the reduced mass region of $[2683,2707]\mevcc$ for the \Omegac data sample collected in 2017\ in the decay-time interval of $[0.9,1.05]\ps$, along with the fit results.  The contributions of the signal, the secondary decays, and the combinatorial background are shown in red (solid), green (dashed), and gray (dash-dotted), respectively.
}
\end{figure}

\begin{figure}[tb]
  \centering
  \includegraphics[width=0.45\linewidth]{Fig8a_S.pdf}
  \includegraphics[width=0.45\linewidth]{Fig8b_S.pdf}
\caption{
Distributions of (left) invariant mass and (right) \logchisqip in the reduced mass region of $[2683,2707]\mevcc$ for the \Omegac data sample collected in 2018\ in the decay-time interval of $[0.52,0.57]\ps$, along with the fit results.  The contributions of the signal, the secondary decays, and the combinatorial background are shown in red (solid), green (dashed), and gray (dash-dotted), respectively.
}
\end{figure}

\begin{figure}[tb]
  \centering
  \includegraphics[width=0.45\linewidth]{Fig9a_S.pdf}
  \includegraphics[width=0.45\linewidth]{Fig9b_S.pdf}
\caption{
Distributions of (left) invariant mass and (right) \logchisqip in the reduced mass region of $[2683,2707]\mevcc$ for the \Omegac data sample collected in 2018\ in the decay-time interval of $[0.9,1.05]\ps$, along with the fit results.  The contributions of the signal, the secondary decays, and the combinatorial background are shown in red (solid), green (dashed), and gray (dash-dotted), respectively.
}
\end{figure}

\begin{figure}[tb]
  \centering
  \includegraphics[width=0.45\linewidth]{Fig10a_S.pdf}
  \includegraphics[width=0.45\linewidth]{Fig10b_S.pdf}
\caption{
Distributions of (left) invariant mass and (right) \logchisqip in the reduced mass region of $[2461,2481]\mevcc$ for the \Xicz data sample collected in 2016\ in the decay-time interval of $[0.52,0.57]\ps$, along with the fit results.  The contributions of the signal, the secondary decays, and the combinatorial background are shown in red (solid), green (dashed), and gray (dash-dotted), respectively.
}
\end{figure}

\begin{figure}[tb]
  \centering
  \includegraphics[width=0.45\linewidth]{Fig11a_S.pdf}
  \includegraphics[width=0.45\linewidth]{Fig11b_S.pdf}
\caption{
Distributions of (left) invariant mass and (right) \logchisqip in the reduced mass region of $[2461,2481]\mevcc$ for the \Xicz data sample collected in 2016\ in the decay-time interval of $[0.69,0.75]\ps$, along with the fit results.  The contributions of the signal, the secondary decays, and the combinatorial background are shown in red (solid), green (dashed), and gray (dash-dotted), respectively.
}
\end{figure}

\begin{figure}[tb]
  \centering
  \includegraphics[width=0.45\linewidth]{Fig12a_S.pdf}
  \includegraphics[width=0.45\linewidth]{Fig12b_S.pdf}
\caption{
Distributions of (left) invariant mass and (right) \logchisqip in the reduced mass region of $[2461,2481]\mevcc$ for the \Xicz data sample collected in 2016\ in the decay-time interval of $[0.9,1.05]\ps$, along with the fit results.  The contributions of the signal, the secondary decays, and the combinatorial background are shown in red (solid), green (dashed), and gray (dash-dotted), respectively.
}
\end{figure}

\begin{figure}[tb]
  \centering
  \includegraphics[width=0.45\linewidth]{Fig13a_S.pdf}
  \includegraphics[width=0.45\linewidth]{Fig13b_S.pdf}
\caption{
Distributions of (left) invariant mass and (right) \logchisqip in the reduced mass region of $[2461,2481]\mevcc$ for the \Xicz data sample collected in 2017\ in the decay-time interval of $[0.52,0.57]\ps$, along with the fit results.  The contributions of the signal, the secondary decays, and the combinatorial background are shown in red (solid), green (dashed), and gray (dash-dotted), respectively.
}
\end{figure}

\begin{figure}[tb]
  \centering
  \includegraphics[width=0.45\linewidth]{Fig14a_S.pdf}
  \includegraphics[width=0.45\linewidth]{Fig14b_S.pdf}
\caption{
Distributions of (left) invariant mass and (right) \logchisqip in the reduced mass region of $[2461,2481]\mevcc$ for the \Xicz data sample collected in 2017\ in the decay-time interval of $[0.69,0.75]\ps$, along with the fit results.  The contributions of the signal, the secondary decays, and the combinatorial background are shown in red (solid), green (dashed), and gray (dash-dotted), respectively.
}
\end{figure}

\begin{figure}[tb]
  \centering
  \includegraphics[width=0.45\linewidth]{Fig15a_S.pdf}
  \includegraphics[width=0.45\linewidth]{Fig15b_S.pdf}
\caption{
Distributions of (left) invariant mass and (right) \logchisqip in the reduced mass region of $[2461,2481]\mevcc$ for the \Xicz data sample collected in 2017\ in the decay-time interval of $[0.9,1.05]\ps$, along with the fit results.  The contributions of the signal, the secondary decays, and the combinatorial background are shown in red (solid), green (dashed), and gray (dash-dotted), respectively.
}
\end{figure}

\begin{figure}[tb]
  \centering
  \includegraphics[width=0.45\linewidth]{Fig16a_S.pdf}
  \includegraphics[width=0.45\linewidth]{Fig16b_S.pdf}
\caption{
Distributions of (left) invariant mass and (right) \logchisqip in the reduced mass region of $[2461,2481]\mevcc$ for the \Xicz data sample collected in 2018\ in the decay-time interval of $[0.52,0.57]\ps$, along with the fit results.  The contributions of the signal, the secondary decays, and the combinatorial background are shown in red (solid), green (dashed), and gray (dash-dotted), respectively.
}
\end{figure}

\begin{figure}[tb]
  \centering
  \includegraphics[width=0.45\linewidth]{Fig17a_S.pdf}
  \includegraphics[width=0.45\linewidth]{Fig17b_S.pdf}
\caption{
Distributions of (left) invariant mass and (right) \logchisqip in the reduced mass region of $[2461,2481]\mevcc$ for the \Xicz data sample collected in 2018\ in the decay-time interval of $[0.9,1.05]\ps$, along with the fit results.  The contributions of the signal, the secondary decays, and the combinatorial background are shown in red (solid), green (dashed), and gray (dash-dotted), respectively.
}
\end{figure}

\begin{figure}[tb]
  \centering
  \includegraphics[width=0.45\linewidth]{Fig18a_S.pdf}
  \includegraphics[width=0.45\linewidth]{Fig18b_S.pdf}
\caption{
Distributions of (left) invariant mass and (right) \logchisqip in the reduced mass region of $[1853,1877]\mevcc$ for the \Dz data sample collected in 2016\ in the decay-time interval of $[0.52,0.57]\ps$, along with the fit results.  The contributions of the signal, the secondary decays, and the combinatorial background are shown in red (solid), green (dashed), and gray (dash-dotted), respectively.
}
\end{figure}

\begin{figure}[tb]
  \centering
  \includegraphics[width=0.45\linewidth]{Fig19a_S.pdf}
  \includegraphics[width=0.45\linewidth]{Fig19b_S.pdf}
\caption{
Distributions of (left) invariant mass and (right) \logchisqip in the reduced mass region of $[1853,1877]\mevcc$ for the \Dz data sample collected in 2016\ in the decay-time interval of $[0.69,0.75]\ps$, along with the fit results.  The contributions of the signal, the secondary decays, and the combinatorial background are shown in red (solid), green (dashed), and gray (dash-dotted), respectively.
}
\end{figure}

\begin{figure}[tb]
  \centering
  \includegraphics[width=0.45\linewidth]{Fig20a_S.pdf}
  \includegraphics[width=0.45\linewidth]{Fig20b_S.pdf}
\caption{
Distributions of (left) invariant mass and (right) \logchisqip in the reduced mass region of $[1853,1877]\mevcc$ for the \Dz data sample collected in 2016\ in the decay-time interval of $[0.9,1.05]\ps$, along with the fit results.  The contributions of the signal, the secondary decays, and the combinatorial background are shown in red (solid), green (dashed), and gray (dash-dotted), respectively.
}
\end{figure}

\begin{figure}[tb]
  \centering
  \includegraphics[width=0.45\linewidth]{Fig21a_S.pdf}
  \includegraphics[width=0.45\linewidth]{Fig21b_S.pdf}
\caption{
Distributions of (left) invariant mass and (right) \logchisqip in the reduced mass region of $[1853,1877]\mevcc$ for the \Dz data sample collected in 2017\ in the decay-time interval of $[0.52,0.57]\ps$, along with the fit results.  The contributions of the signal, the secondary decays, and the combinatorial background are shown in red (solid), green (dashed), and gray (dash-dotted), respectively.
}
\end{figure}

\begin{figure}[tb]
  \centering
  \includegraphics[width=0.45\linewidth]{Fig22a_S.pdf}
  \includegraphics[width=0.45\linewidth]{Fig22b_S.pdf}
\caption{
Distributions of (left) invariant mass and (right) \logchisqip in the reduced mass region of $[1853,1877]\mevcc$ for the \Dz data sample collected in 2017\ in the decay-time interval of $[0.69,0.75]\ps$, along with the fit results.  The contributions of the signal, the secondary decays, and the combinatorial background are shown in red (solid), green (dashed), and gray (dash-dotted), respectively.
}
\end{figure}

\begin{figure}[tb]
  \centering
  \includegraphics[width=0.45\linewidth]{Fig23a_S.pdf}
  \includegraphics[width=0.45\linewidth]{Fig23b_S.pdf}
\caption{
Distributions of (left) invariant mass and (right) \logchisqip in the reduced mass region of $[1853,1877]\mevcc$ for the \Dz data sample collected in 2017\ in the decay-time interval of $[0.9,1.05]\ps$, along with the fit results.  The contributions of the signal, the secondary decays, and the combinatorial background are shown in red (solid), green (dashed), and gray (dash-dotted), respectively.
}
\end{figure}

\begin{figure}[tb]
  \centering
  \includegraphics[width=0.45\linewidth]{Fig24a_S.pdf}
  \includegraphics[width=0.45\linewidth]{Fig24b_S.pdf}
\caption{
Distributions of (left) invariant mass and (right) \logchisqip in the reduced mass region of $[1853,1877]\mevcc$ for the \Dz data sample collected in 2018\ in the decay-time interval of $[0.52,0.57]\ps$, along with the fit results.  The contributions of the signal, the secondary decays, and the combinatorial background are shown in red (solid), green (dashed), and gray (dash-dotted), respectively.
}
\end{figure}

\begin{figure}[tb]
  \centering
  \includegraphics[width=0.45\linewidth]{Fig25a_S.pdf}
  \includegraphics[width=0.45\linewidth]{Fig25b_S.pdf}
\caption{
Distributions of (left) invariant mass and (right) \logchisqip in the reduced mass region of $[1853,1877]\mevcc$ for the \Dz data sample collected in 2018\ in the decay-time interval of $[0.9,1.05]\ps$, along with the fit results.  The contributions of the signal, the secondary decays, and the combinatorial background are shown in red (solid), green (dashed), and gray (dash-dotted), respectively.
}
\end{figure}

\clearpage
